# Supplementary material for: Generalised Unsupervised Domain Adaptation of Neural Machine Translation with Cross-Lingual Data Selection
Source: arXiv:2109.04292 source file (2021-09-09)
Supplement: Supplementary file 1 [file tab-appendix-sel.tex]

\begin{table*}[!h]
\begin{center}
\scalebox{0.6}{
\begin{tabular}{l||rrrrrr|rrrrrr|rrrrrr}
\toprule
 & \multicolumn{6}{c|}{\textbf{Fr-En} (33.70)} & \multicolumn{6}{c}{\textbf{De-En} (31.31)}  & \multicolumn{6}{|c}{\textbf{Cs-En} (25.30)}\\
\multicolumn{1}{c||}{} & 
\multicolumn{1}{c}{law} & \multicolumn{1}{c}{med} & \multicolumn{1}{c}{IT} & \multicolumn{1}{c}{Koran} & \multicolumn{1}{c}{TED} & \multicolumn{1}{c|}{Patent} &
\multicolumn{1}{c}{law} & \multicolumn{1}{c}{med} & \multicolumn{1}{c}{IT} & \multicolumn{1}{c}{Koran} & \multicolumn{1}{c}{TED} & \multicolumn{1}{c|}{Patent} &
\multicolumn{1}{c}{law} & \multicolumn{1}{c}{med} & \multicolumn{1}{c}{IT} & \multicolumn{1}{c}{Koran} & \multicolumn{1}{c}{TED} & \multicolumn{1}{c}{Patent} 
\\
\midrule
zero-shot & \\
\midrule
random &  \\
% n-gram & \\
CED &  \\
domain-finetune & \\
constrastive &  \\ 
\midrule
supervised learning &  \\
\bottomrule
\end{tabular}
}
\caption{Data selection result to English where in-domain source language sentences are available. \todo{Select up to 12M tokens, or 500K sentences}}
\label{tab:result-to-en}
\end{center}
\end{table*}

\begin{table*}[!h]
\begin{center}
\scalebox{0.6}{
\begin{tabular}{l||rrrrrr|rrrrrr|rrrrrr}
\toprule
 & \multicolumn{6}{c|}{\textbf{En-Fr}} & \multicolumn{6}{c}{\textbf{En-De}}  & \multicolumn{6}{|c}{\textbf{En-Cs} (20.75)}\\
\multicolumn{1}{c||}{} & 
\multicolumn{1}{c}{law} & \multicolumn{1}{c}{med} & \multicolumn{1}{c}{IT} & \multicolumn{1}{c}{Koran} & \multicolumn{1}{c}{TED} & \multicolumn{1}{c|}{Patent} &
\multicolumn{1}{c}{law} & \multicolumn{1}{c}{med} & \multicolumn{1}{c}{IT} & \multicolumn{1}{c}{Koran} & \multicolumn{1}{c}{TED} & \multicolumn{1}{c|}{Patent} &
\multicolumn{1}{c}{law} & \multicolumn{1}{c}{med} & \multicolumn{1}{c}{IT} & \multicolumn{1}{c}{Koran} & \multicolumn{1}{c}{TED} & \multicolumn{1}{c|}{Patent} 
\\
\midrule
zero-shot & \\
\midrule
random & \\
% n-gram & \\
CED & \\
domain-finetune & \\
constrastive & \\
\midrule
supervised learning & \\
\bottomrule
\end{tabular}
}
\caption{Data selection result from English where in-domain target language sentences are available.}
\label{tab:result-from-en}
\end{center}
\end{table*}
